# Supplementary material for: Plasma Wave Seed for Raman Amplifiers
Source: arXiv:1612.06450 source file (2017-04-10)
Supplement: Supplementary file 1 [file RamanAmpPl_suppl.pdf]

# Supplemental Materials: Plasma Wave Seed for Raman Amplifiers

Kenan Qu, Ido Barth, and Nathaniel J. Fisch

*Department of Astrophysical Sciences, Princeton University, Princeton, New Jersey 08544, USA*

## I. DERIVATION OF GREEN'S FUNCTIONS

In this section, we solve the linear stage of the coupled three-wave equations using Laplace transform. When the pump depletion can be neglected, Eqs. (1) in the main text reduce to

$$b_t + cb_z = \gamma_0 f^*, \quad f_t = \gamma_0 b^*, \quad (\text{S1})$$

where  $\gamma_0 = aV$  and the initial conditions are  $f(t=0) = f_0$ ,  $b(t=0) = b_0$ . Since this is a coupled first order differential equation with initial value at  $t=0$ , we take the Laplace transform in the time domain

$$\mathfrak{L}[b_t] = sB(s) - b_0, \quad \mathfrak{L}[f_t] = sF(s) - f_0. \quad (\text{S2})$$

Eqs. (S1) transform to the  $s$  domain as

$$sB - b_0 + cB_z = \gamma_0 F^*, \quad sF - f_0 = \gamma_0 B^*. \quad (\text{S3})$$

By eliminating  $F$  we obtain

$$cB_z + \frac{s^2 - \gamma_0^2}{s} B - \frac{\gamma_0}{s} f_0^* - b_0 = 0. \quad (\text{S4})$$

Solving this differential equations with respect to  $z$  yields

$$B = \int \frac{dz'}{c} \left[ \frac{\gamma_0}{s} f_0^*(z') + b_0(z') \right] e^{-\frac{s^2 - \gamma_0^2}{cs}(z - z')}. \quad (\text{S5})$$

For the inverse Laplace transform, we use identities

$$\mathfrak{L}^{-1}[G(s)H(s)] = g(t) * h(t) \equiv \int_0^t g(t')h(t-t')dt', \quad (\text{S6})$$

$$\mathfrak{L}^{-1}[e^{-as}] = \delta(t-a), \quad (\text{S7})$$

$$\mathfrak{L}^{-1}\left[\frac{1}{s}e^{\frac{a}{s}}\right] = I_0(2\sqrt{at}), \quad (\text{S8})$$

$$\mathfrak{L}^{-1}\left[e^{\frac{a}{s}}\right] = \sqrt{\frac{a}{t}}I_1(2\sqrt{at}) + \delta(t). \quad (\text{S9})$$

So that

$$\begin{aligned} \mathfrak{L}^{-1}[e^{-s(z-z')/c}] &= \delta(t - z/c + z'/c), \\ \mathfrak{L}^{-1}\left[\frac{1}{s}e^{\frac{\gamma_0^2}{cs}(z-z')}\right] &= I_0[2\gamma_0\sqrt{t(z-z')/c}], \\ \mathfrak{L}^{-1}\left[e^{\frac{\gamma_0^2}{cs}(z-z')}\right] &= \sqrt{\frac{\gamma_0^2(z-z')}{ct}}I_1(2\gamma_0\sqrt{t(z-z')/c}) + \delta(t). \end{aligned} \quad (\text{S10})$$

Therefore,

$$\begin{aligned} &\mathfrak{L}^{-1}\left[\frac{1}{s}e^{-\frac{s^2 - \gamma_0^2}{cs}(z-z')}\right] \\ &= \mathfrak{L}^{-1}\left[\frac{1}{s}e^{\frac{\gamma_0^2}{cs}(z-z')}e^{-s(z-z')/c}\right] \\ &= \mathfrak{L}^{-1}\left[\frac{1}{s}e^{\frac{\gamma_0^2}{cs}(z-z')}\right] * \mathfrak{L}^{-1}[e^{-s(z-z')/c}] \\ &= I_0[2\gamma_0\sqrt{t(z-z')/c}] * \delta(t - z/c + z'/c) \\ &= I_0[2\gamma_0\sqrt{(\frac{z}{c} - \frac{z'}{c})(t - \frac{z}{c} + \frac{z'}{c})}] \cdot \Theta(t - \frac{z}{c} + \frac{z'}{c}), \end{aligned} \quad (\text{S11})$$

and

$$\begin{aligned}
& \mathfrak{L}^{-1}[e^{-\frac{s^2 - \gamma_0^2}{cs}(z-z')}] \\
&= \mathfrak{L}^{-1}[e^{\frac{\gamma_0^2}{cs}(z-z')} e^{-s(z-z')/c}] \\
&= \mathfrak{L}^{-1}[e^{\frac{\gamma_0^2}{cs}(z-z')}] * \mathfrak{L}^{-1}[e^{-s(z-z')/c}] \\
&= \left\{ \sqrt{\frac{\gamma_0^2(z-z')}{ct}} I_1[2\gamma_0 \sqrt{t(z-z')/c}] + \delta(t) \right\} * \delta(t - z/c + z'/c) \\
&= \sqrt{\frac{\gamma_0^2(z-z')}{ct - z + z'}} I_1[2\gamma_0 \sqrt{(\frac{z}{c} - \frac{z'}{c})(t - \frac{z}{c} + \frac{z'}{c})}] \cdot \Theta(t - \frac{z}{c} + \frac{z'}{c}) + \delta(t - \frac{z}{c} + \frac{z'}{c}), \tag{S12}
\end{aligned}$$

The solution to  $b$  is

$$\begin{aligned}
b(t, z) &= \int dz' [G_{\text{bf}}(t, z - z') f_0^*(z') + G_{\text{bb}}(t, z - z') b_0(z')], \\
G_{\text{bf}}(t, z) &= \frac{\gamma_0}{c} I_0[2\gamma_0 \sqrt{\frac{z}{c}(t - \frac{z}{c})}] \cdot \Theta(t - \frac{z}{c}), \\
G_{\text{bb}}(t, z) &= \frac{\gamma_0}{c} \sqrt{\frac{z}{ct - z}} I_1[2\gamma_0 \sqrt{\frac{z}{c}(t - \frac{z}{c})}] \cdot \Theta(t - \frac{z}{c}) + \frac{1}{c} \delta(t - \frac{z}{c}). \tag{S13}
\end{aligned}$$

## II. AMPLIFICATION OF A SEED WITH A FINITE DURATION

Beyond the linear regime, as the probe pulse propagates and grows, it should begin to deplete the pump and enter into the nonlinear stage. Its nonlinear dynamics is governed by Eqs. (1) which, unfortunately, do not have a general solution to our knowledge. Derivation of the “ $\pi$ -pulse” solution [S1], however, automatically assumes a single variable dependence on  $z(ct - z)$ , ignoring any initial distribution of plasma or laser seeds. On the other hand, the variable  $z(ct - z)$  by itself indicates that the wavefront of the probe beam (close to  $ct - z \sim 0$ ) asymptotically determines the nonlinear dynamics at large  $z$ . The asymptotic equivalence expressed in Eq. (7) in the main text suggests that a plasma seed with the shape of derivative of a delta function, *i.e.*,  $(c/\gamma_0)\delta'(z)$ , should generate a delta-function-shape probe beam in the linear stage, and eventually yield a “ $\pi$ -pulse” structure in the nonlinear regime. Nevertheless, we cannot rule out other types of plasma seeds which may also yield “ $\pi$ -pulse” solutions.

Practically, any seed has a distribution with a finite width. Next, we find the condition of the plasma seed shape for continued amplification. We define the spatial growth rate along propagating length  $z$  as  $\gamma(\zeta) = b_z/b$ , which also differentiates the growth rate for its different parts  $\zeta = ct - z$ . Assuming the most advanced part of the probe beam is small and pump is not depleted, Eqs. (1) in the main text transform to  $cb_z = \gamma_0 f^*$  and  $cf_\zeta = \gamma_0 b^*$ . By substitution, we get the wavefront growth rate  $\gamma = (\gamma_0/c)^2 / \partial_\zeta(\ln f^*)$ . Then  $\gamma_\zeta = -(\gamma_0/c)^2 \partial_{\zeta\zeta}(\ln f^*) / [\partial_\zeta(\ln f^*)]^2$ . We argue that the sharpness of probe wavefront increases if the spatial growth rate is large close to the probe peak and lower far from the rising edge. In another word, the growth rate increases from the far end to the peak position, *i.e.*,  $\gamma_\zeta > 0$  around  $\zeta \sim 0$ , or equivalently  $\partial_{\zeta\zeta}(\ln f_0^*) < 0$ . Therefore, any seeds whose wavefront envelope is equal to, or sharper than, a Gaussian shape with a finite width will continue to contract and gets amplified much resembling a “ $\pi$ -pulse”. This is reminiscent of suppressing the superluminal precursors requiring the laser seed be sharper than Gaussian [S2]. Physically, this can be attributed to the nonlinear amplification property of the Green’s function  $G_{\text{bf}}$ . It suppresses the rising edge (at smaller  $\zeta$ ) of the seed while amplifying its peak component (at larger  $\zeta$ ), allowing probe beam to maintain its sharpness.

## III. PIC SIMULATIONS WITH A HIGHER TEMPERATURE

Although the parametric interaction in a PIC simulation changes with temperature [S3] effecting the numerically calculated Raman growth rate, this change is identical whether we consider the plasma wave seed or the laser seed. To show this, we conduct the PIC simulations by increasing the plasma temperature to 50 eV. We keep other parameters the same as in Fig. (3) in the main text. With the elevated temperature, the amplified pulses using different seeds remain in good agreements for both the leading peak envelopes [Fig. S1(b)] and the maximum intensity [Fig. S1(c)]. Fig. S1(a) displays the early stage of amplification. Compared with the results in Fig. (3), the probe beam scattered

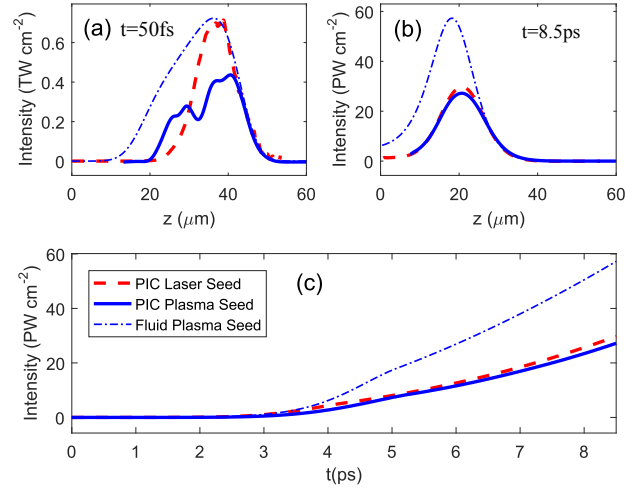

FIG. S1. Comparison of Raman amplification using a plasma seed (blue solid line) and a laser seed (red dashed line). The electron temperature is set to 50 eV. (a) and (b) show the amplified probe pulses at interaction time  $t = 50$ fs and  $t = 8.5$ ps, respectively. (c) Comparison of the amplified probe pulse peak intensity. The thick solid and dashed lines are PIC simulations; and the thin dotted-dash lines are fluid-model simulations using Eqs.(1) in the main text.

from a Langmuir wave seed shows a lower peak intensity and that from a laser seed shows a shorter amplified tail. They together reveal a reduced interaction rate at a higher temperature (50 eV). For the same parameters, the peak intensity of amplified pulse at 8.5ps is  $40 \text{ PW cm}^{-2}$  at 10 eV, while it drops to about  $30 \text{ PW cm}^{-2}$  at 50 eV.

- 
- [S1] V. M. Malkin, G. Shvets, and N. J. Fisch, “Fast compression of laser beams to highly overcritical powers,” *Phys. Rev. Lett.* **82**, 4448 (1999).
  - [S2] Yu. A. Tsidulko, V. M. Malkin, and N. J. Fisch, “Suppression of superluminous precursors in high-power backward Raman amplifiers,” *Phys. Rev. Lett.* **88**, 235004 (2002).
  - [S3] M. R. Edwards, Z. Toroker, J. M. Mikhailova, and N. J. Fisch, “The efficiency of Raman amplification in the wavebreaking regime,” *Phys. Plasmas* **22**, 074501 (2015).
